# Supplementary material for: Learning Task Knowledge and its Scope of Applicability in Experience-Based Planning Domains
Source: arXiv:1902.10770 source file (2019-03-05)
Supplement: Supplementary file 1 [file appendix.tex]

\appendix
\section{Contiguous Non-overlapping Longest Common Prefix Array}
\label{sec:app}

Here we present an updated version of the $CNLCP$ algorithm 
\cite{vahid2017iros,vahid2017prletter} for computing potential 
patterns in a string. 
Given a string (representing the abstract plan $\Omega$ of a generalized and 
abstracted experience), Algorithm~\ref{alg:cnlcp} builds the suffix array $SA$, 
the $NLCP$ array, and the $CNLCP$ array for the string.

Let \texttt{'abacacacdedfdfgh'} be the string representing the abstract plan 
of the activity schema in Listing~\ref{lst:schema}. 
Table~\ref{tbl:nlcp} shows the computed $SA$ and $NLCP$ arrays, and 
Table~\ref{tbl:cnlcp} shows the computed $CNLCP$ array for this string. 
$CNLCP$ gives the patterns (iterations of loops) \texttt{ac} and \texttt{df} 
happening at the positions ($2$, $4$, $6$) and ($10$, $12$) respectively. 
The resulting looping string is \ttf{ab(ac)$^*$de(df)$^*$gh}. 

%---------------------------------------------------------------------------

%---------------------------------------------------------------------------
\begin{algorithm}[t]
\caption{Contiguous Non-overlapping Longest Common Prefixes ($CNLCP$)}
\label{alg:cnlcp}
\begin{algorithmic}[1]
{
\Require $\Omega$
    \Comment{{\scriptsize a string (representing the enriched abstract plan of an activity schema)}}
\Ensure $CNLCP$
    \Comment{{\scriptsize a contiguous non-overlapping longest common prefixes array (Def.~\ref{def:cnlcp})}}

  \vspace{10pt}
  \State $SA \gets \ttf{sorted}(\ttf{range}(\ttf{len}(\Omega)),\ttf{key}=lambda~i: \Omega[i:])$
  \label{alg:cnlcs:sa}
  \Comment{{\scriptsize build a suffix array from $\Omega$ (in python)}}
  \State $NLCP[0] \gets 0$
  \For {$i$ in $\ttf{range}(\ttf{len}(SA)-1)$}
  \Comment{{\scriptsize build a non-overlapping longest 
  common prefixes array, NLCP (Def.~\ref{def:nlcpa})}}
      \State $NLCP[i+1] \gets \Call{\ttf{nlcp}}
      {\Omega[SA[i]:],\Omega[SA[i+1]:]}$\label{alg:cnlcs:nlcs}
      \Comment{{\scriptsize see line \ref{alg:nlcp:function}}}
  \EndFor
%  \State $nlcp \gets$ \Call{NLCPArray}{$sa,\Omega$}
  \State $CNLCP~\gets \EmpSet$\label{alg:cnlcs:cnlcp:st}
  \Comment{{\scriptsize an empty dictionary}} 
  \For {$maxlen$ in $\ttf{sorted}($NLCP$)$}
  \Comment{{\scriptsize build a CNLCP array (Def.~\ref{def:cnlcp})}}
       \For {$i$ in $\ttf{range}(\ttf{len}(\Omega))$} 
           \If {$NLCP[i] == maxlen$ }
              \If {$\ttf{abs}(SA[i]-SA[i-1]) == maxlen$}
              \label{alg:cnlcp:if}
              \Comment{{\scriptsize keep only consecutive occurrences in NLCP}}
                \State $k~\gets \Omega[SA[i]:SA[i]+maxlen]$
                % \Comment{{\scriptsize a possible pattern}}
                \State $CNLCP[k]~\gets$ $CNLCP[k] \cup \{SA[i-1]\}$
                \label{alg:cnlcs:cnlcp:en}
                \Comment{{\scriptsize starting position of pattern $k$}}
              \EndIf
           \EndIf\vspace{-1.6pt}
       \EndFor
  \EndFor
\State \Return $CNLCP$
\vspace{20pt}

\Function{$\ttf{nlcp}$}{$suf_1,suf_2$}\label{alg:nlcp:function}
 \Comment{{\scriptsize find the non-overlapping longest 
    common prefix between two given suffixes (Def.~\ref{def:nlcp})}}
 \State $maxlen \gets \ttf{min}(\ttf{abs}(\ttf{len}(suf_1)-\ttf{len}(suf_2)),\ttf{len}(suf_1),\ttf{len}(suf_2))$
 \label{alg:lcp:max}
 \For {$i$ in $\ttf{range}(maxlen)$} 
     \If {$suf_1[i] \neq suf_2[i]$ }
        \State \Return $\ttf{len}(suf_1[0:i])$
     \EndIf
 \EndFor
  \vspace{-2pt}
 \State \Return $\ttf{len}(suf_1[0:maxlen])$
\EndFunction

}%font size
\end{algorithmic}
\end{algorithm}
%---------------------------------------------------------------------------

%%%%%%%%%%%%%%%%%%%%%%%%%%%%%%%%%%%%%%%%%%%%%%%%%%%%%%%%%%%
\begin{table}[t]
%\vspace{-5pt}
%\setlength{\tabcolsep}{10pt}
  \centering
  \caption{The computed $SA$ and $NLCP$ arrays for the 
  string \texttt{'abacacacdedfdfgh'}.}
  %\resizebox{\columnwidth}{!}
  {
  \begin{tabular}{clcc}
  $i$ & suffix & $SA[i]$ & $NLCP[i]^*$ \\
    \hline
    0 & \ttf{abacacacdedfdfgh} & 0  & 0 \\
    1 & \ttf{acacacdedfdfgh}   & 2  & 1 \\
    2 & \ttf{acacdedfdfgh}     & 4  & 2 \\
    3 & \ttf{acdedfdfgh}       & 6  & 2 \\
    4 & \ttf{bacacacdedfdfgh}  & 1  & 0 \\
    5 & \ttf{cacacdedfdfgh}    & 3  & 0 \\
    6 & \ttf{cacdedfdfgh}      & 5  & 2 \\
    7 & \ttf{cdedfdfgh}        & 7  & 1 \\
    8 & \ttf{dedfdfgh}         & 8  & 0 \\
    9 & \ttf{dfdfgh}           & 10 & 1 \\
   10 & \ttf{dfgh}             & 12 & 2 \\
   11 & \ttf{edfdfgh}          & 9  & 0 \\
   12 & \ttf{fdfgh}            & 11 & 0 \\
   13 & \ttf{fgh}              & 13 & 1 \\
   14 & \ttf{gh}               & 14 & 0 \\
   15 & \ttf{h}                & 15 & 0 \\\hline
  \end{tabular}
  }
  {\begin{flushleft}
   \scriptsize \ \ 
   $^{\rm *}$
   {Each number in $i^{\text{th}}$ row specifies the 
    length of the non-overlapping longest common prefix 
    between two suffixes in rows $i$ and $(i-1)$ for $i\geq1$.
    For example, in rows $1$ and $2$, \texttt{'ac'} is the 
    non-overlapping longest common prefix between two consecutive 
    suffixes \texttt{'acacacdedfdfgh'} and \texttt{'acacdedfdfgh'}.}
  \end{flushleft}}
\label{tbl:nlcp}
%\vspace{-5pt}
\end{table}
%%%%%%%%%%%%%%%%%%%%%%%%%%%%%%%%%%%%%%%%%%%%%%%%%%%%%%%%%%%

%%%%%%%%%%%%%%%%%%%%%%%%%%%%%%%%%%%%%%%%%%%%%%%%%%%%%%%%%%%
\begin{table}[t]
%\vspace{-5pt}
%\setlength{\tabcolsep}{10pt}
  \centering
  \caption{The computed $CNLCP$ array for the same 
  string \texttt{'abacacacdedfdfgh'}.}
  %\vspace{-5pt}
  %\resizebox{\columnwidth}{!}
  % \footnotesize
  {
  \begin{tabular}{ll}
  $k$ & $CNLCP[k]$ \\
    \hline
  \ttf{ac} & 2, 4, 6 \\
  \ttf{df} & 10, 12 \\
%  \st{1} & \st{aB} & \st{1, 5} \\
%   1 & B & 2, 6 \\
%  \st{1} & \st{b} & \st{1, 3} \\ 
  \hline
  \end{tabular}
  }
  \begin{flushleft}
  \scriptsize \ \ 
  Each substring in the CNLCP array is a pattern (an iteration of 
  a loop) with its starting positions in a given string.
  \end{flushleft}
\label{tbl:cnlcp}
%\vspace{-5pt}
\end{table}
%%%%%%%%%%%%%%%%%%%%%%%%%%%%%%%%%%%%%%%%%%%%%%%%%%%%%%%%%%%
